# Supplementary material for: Coercivity-size map of magnetic nanoflowers: spin disorder tunes the vortex reversal mechanism and tailors the hyperthermia sweet spot
Source: arXiv:2507.02154 source file (2025-07-02)
Supplement: Supplementary file 1 [file supplemental_arxiv.pdf]

# Supporting Information to: Coercivity-size map of magnetic nanoflowers: spin disorder tunes the vortex reversal mechanism and tailors the hyperthermia sweet spot

Elizabeth M. Jefremovas,<sup>1,2,\*</sup> Lisa Calus,<sup>3</sup> and Jonathan Leliaert<sup>3,†</sup>

<sup>1</sup>*Department of Physics and Materials Science, University of Luxembourg,  
162A Avenue de la Faiencerie, L-1511 Luxembourg, Grand Duchy of Luxembourg*

<sup>2</sup>*Institute for Advanced Studies, University of Luxembourg,  
Campus Belval, L-4365 Esch-sur-Alzette, Luxembourg*

<sup>3</sup>*DyNaMat, Department of Solid State Sciences, Ghent University, 9000 Ghent, Belgium*

This Supporting Information contains extended technical details on the simulations (S1); the full hysteresis loops for selected sizes (S2); the coercivity vs. nanoflower size mapping considering a multi-grain structure for all NF sizes (S3); extended discussion on the determination of the net magnetization direction of the magnetic nanoparticles (S4); the magnetization reversal studied in the case of perfect nanospheres; and the  $k = 0$  case for the influence of intra-particle disorder.

## I. SIMULATION DETAILS

Numerical simulations were performed using Mumax3 [1], an open-source GPU-accelerated micromagnetic simulation program. The software solves the time- and space- dependent magnetization evolution, described by the Landau-Lifshitz-Gilbert equation, in nano- to micro-scale magnets using a finite-difference discretization. We refer to Ref. [1] for a detailed description of the physical model implemented, and instead focus below on the technical details of the simulations we performed.

The nanoflowers were generated from a perfectly spherical geometry with an initial diameter of  $d = 10 - 400$  nm. A Voronoi tessellation was applied to this sphere to define discrete regions [2], corresponding to individual material grains. The grains with Voronoi centers laying inside the base sphere were kept in their entirety (also extending outside the sphere), whereas areas of grains whose Voronoi center lays outside of the sphere were completely discarded. This results in the non-spherical flower shape as seen in the inset of Figure 1 of the main paper. We checked that the average volume of the randomly generated geometries coincides with that of the sphere, thus resulting in the same effective diameter. Each grain was assigned a randomly oriented anisotropy axis to reproduce the polycrystalline nature typically observed in experimentally synthesized nanoflowers [3–6].

To reproduce the effect of intra-particle disorder, the magnetic coupling between adjacent grains was modeled by rescaling the exchange stiffness parameter  $A$  at the grain boundaries by a factor  $k$  lying between 0 and 1. We find good agreement with the experimental results for  $k = 0.25$  [3, 4, 6, 7]. Material parameters typical for iron oxide were used based on literature. These include saturation magnetization  $M_s = 400 \times 10^3$  A/m [8, 9],

exchange stiffness  $A = 10$  pJ/m [10], and uniaxial magnetocrystalline anisotropy  $K_u = 10^4$  J/m<sup>3</sup> [8, 11–13]. Each simulated size has been realized between 15-25 times with a different random seed for the Voronoi tessellation to ensure the statistical significance of our results.

We have adjusted the cell size and number of cells depending on the nanoflower size, the grain texture and the material parameters. First, the exchange length of our material is  $l_{ex} = \sqrt{\frac{A}{\mu_0 M_s^2}} \cong 7.052$  nm, setting the upper limit for our cell size. We have benchmarked a collection of cell sizes from 1.500 to 5.000 nm in steps of 0.125 nm, finding, for the same field step, a factor 3 performance difference between the smallest and the largest discretization cells. Considering the amount of simulations performed in this work, we fixed the cell size as a function of the nanoflower diameter to maximize the compromise between accuracy and computing time. The number of cells was varied depending on the nanoflower diameter to keep the grid size dimensions *7-smooth*. The values and cell dimensions are included in the following table.

TABLE I. Nanoflower diameter, cell size and number of cells  $N$  used for each realization

| $\bar{d}$ (nm) | cell size (nm) | $N$     |
|----------------|----------------|---------|
| 10 – 15        | 1.125          | $16^3$  |
| 17 – 20        | 1.125          | $24^3$  |
| 22 – 30        | 1.125          | $32^3$  |
| 32 – 48        | 1.125          | $48^3$  |
| 50 – 70        | 3.125          | $32^3$  |
| 72 – 100       | 3.125          | $48^3$  |
| 110 – 140      | 5.000          | $32^3$  |
| 150 – 200      | 5.000          | $48^3$  |
| 210 – 280      | 5.000          | $64^3$  |
| 290 – 400      | 5.000          | $128^3$ |

For  $d \leq 50$  nm, the grain size was reduced from 15 nm to 5 nm, setting one random anisotropy direction for all grains (all grains following the same  $K_u$ ) with fixed  $k = 1$ , to reproduce the single-domain behavior.

\* elizabeth.jefremovas@uni.lu

† jonathan.leliaert@ugent.be

In addition to the nanoflower geometry, we have also simulated the case of idealized spherical particles with uniform geometry, no grain boundaries, and a single anisotropy axis ( $K_u$ ) aligned along  $z$ . The realizations follow the same cell size and  $N$  indicated in Table I.

The main parameter shown in this study is the coercive field  $\mu_0 H_C$ , which is extracted from the hysteresis loop. For simulating these loops, we initialized the magnetization at saturation ( $\mu_0 H_z = 1.2$  T). The field is then reduced in a stepwise fashion to  $\mu_0 H_z = -0.1$  T, first in steps of  $-2.5$  mT from saturation to  $\mu_0 H_z = 0.1$  T, and then, in finer steps of  $-0.1$  mT to fully capture the switching of the magnetization. In each step, we minimize the total energy of the system by using the *relax()* function of Mumax3, which solves the Landau-Lifshitz-Gilbert equation without precession.

### A. Simulation hardware

Most simulations were run on the Tier 1 supercomputer (Hortense) of the Flemish supercomputer center within a Tier-1 compute project. The simulations consumed 40,000 GPU-hours on 80 NVIDIA A100 GPU's over an 8 month period. In addition, we made use of the Tier 2 GPU infrastructure of both Ghent University and the University of Luxembourg, both providing NVIDIA V100 GPU's, and the Tier 1 Luxembourg national supercomputer MeluXina, providing NVIDIA A100 GPU's.

## II. HYSTERESIS LOOPS FOR SELECTED SIZES

Figure 1 includes the complete hysteresis loops for  $d = 30$  nm,  $d = 70$  nm,  $d = 100$  nm, and  $d = 120$  nm. 20 different random initial configurations per NF size are performed to ensure that the average result is statistically significant. The middle panel includes the average of the seeds, from which the coercivity is extracted. On the right hand side panel we have included the equatorial planes for each configuration at remanence. The evolution from single domain ( $d = 30$  nm) to domain wall ( $d = 70$  nm) and a vortex pointing along the  $z$  direction ( $d = 100$ , and 120 nm) can be inspected.

### III. SINGLE GRAIN MODEL VALIDATION FOR SMALL NANOFLOWERS

In Figure 1 of the main text, we showed the results of the simulations modeling the single-domain region with a single grain nanoflower, meaning,  $N = 1$ , which comprises the whole nanoflower. This procedure is consistent with the single-domain nature of the NF. If instead, the granular texture is maintained, with a fixed grain size of 15 nm, the obtained results are compatible with the ones of single domain, but indeed, with an increased noise. Figure 2 (A) includes the results, considering a

fixed grain size of 15 nm, for the coercivity as a function of the NF diameter  $d$ . As it can be observed, within the error bars, the results corresponding to the single domain region ( $d < 50$  nm) are compatible with the ones included in the main text when a single-grain is considered, yet they carry a non-negligible noise due to the different geometry realizations. Indeed, the irregular shape of the NFs, together with the grain size itself (15 nm) make it impossible to accommodate all grains without sharp cuts, and also result in relatively large volume differences between different realizations of the geometry. As a consequence, some of the realizations do not display a nanoflower morphology, but rather unphysical “incomplete grain assemblies”, as can be seen in the snapshots included in Figure 2 (B) for sizes up to  $d = 70$  nm. As a reference, the ones for  $d = 90$  and 110 nm conform much more to the real nanoflower geometries.

To avoid any effects of unphysical geometries, we modified our simulations to model the single-domain region without an internal grain structure.

## IV. RATIO VORTEX CORE VS. NANOPARTICLE VOLUME

Figure 2 (E) of the main text shows the ratio between the vortex core volume *vs.* total nanoparticle volume. We found a change in the magnetization reversal modes when the core volume fell below 1/3rd of the total volume.

To obtain the total volume of the nanoflowers with irregular geometry, we accessed the magnetization vector  $\vec{m} = (m_x, m_y, m_z)$  at each simulation cell and multiplied the non-zero vectors by the corresponding cell size.

To quantify the core volume, we proceed in three steps. First, we average all cell magnetization vectors and normalize this average to define the unit vector  $\hat{m}_{\text{net}}$ , representing the overall magnetization direction. Next, for every cell we take the dot product between its magnetization  $\vec{m}$  and  $\hat{m}_{\text{net}}$ ; this yields a weight from -1 to +1 that measures how closely the cell aligns with the net direction. Cells with negative weights are counter-aligned, so we set their contribution to zero. Finally, we sum the volumes of the remaining cells, each multiplied by its positive weight, thereby obtaining an estimate of the vortex-core volume.

## V. MAGNETIZATION REVERSAL IN PERFECT SPHERES

In Figure 2 of the main text, we elucidate two regimes for the magnetization reversal, depending on whether the

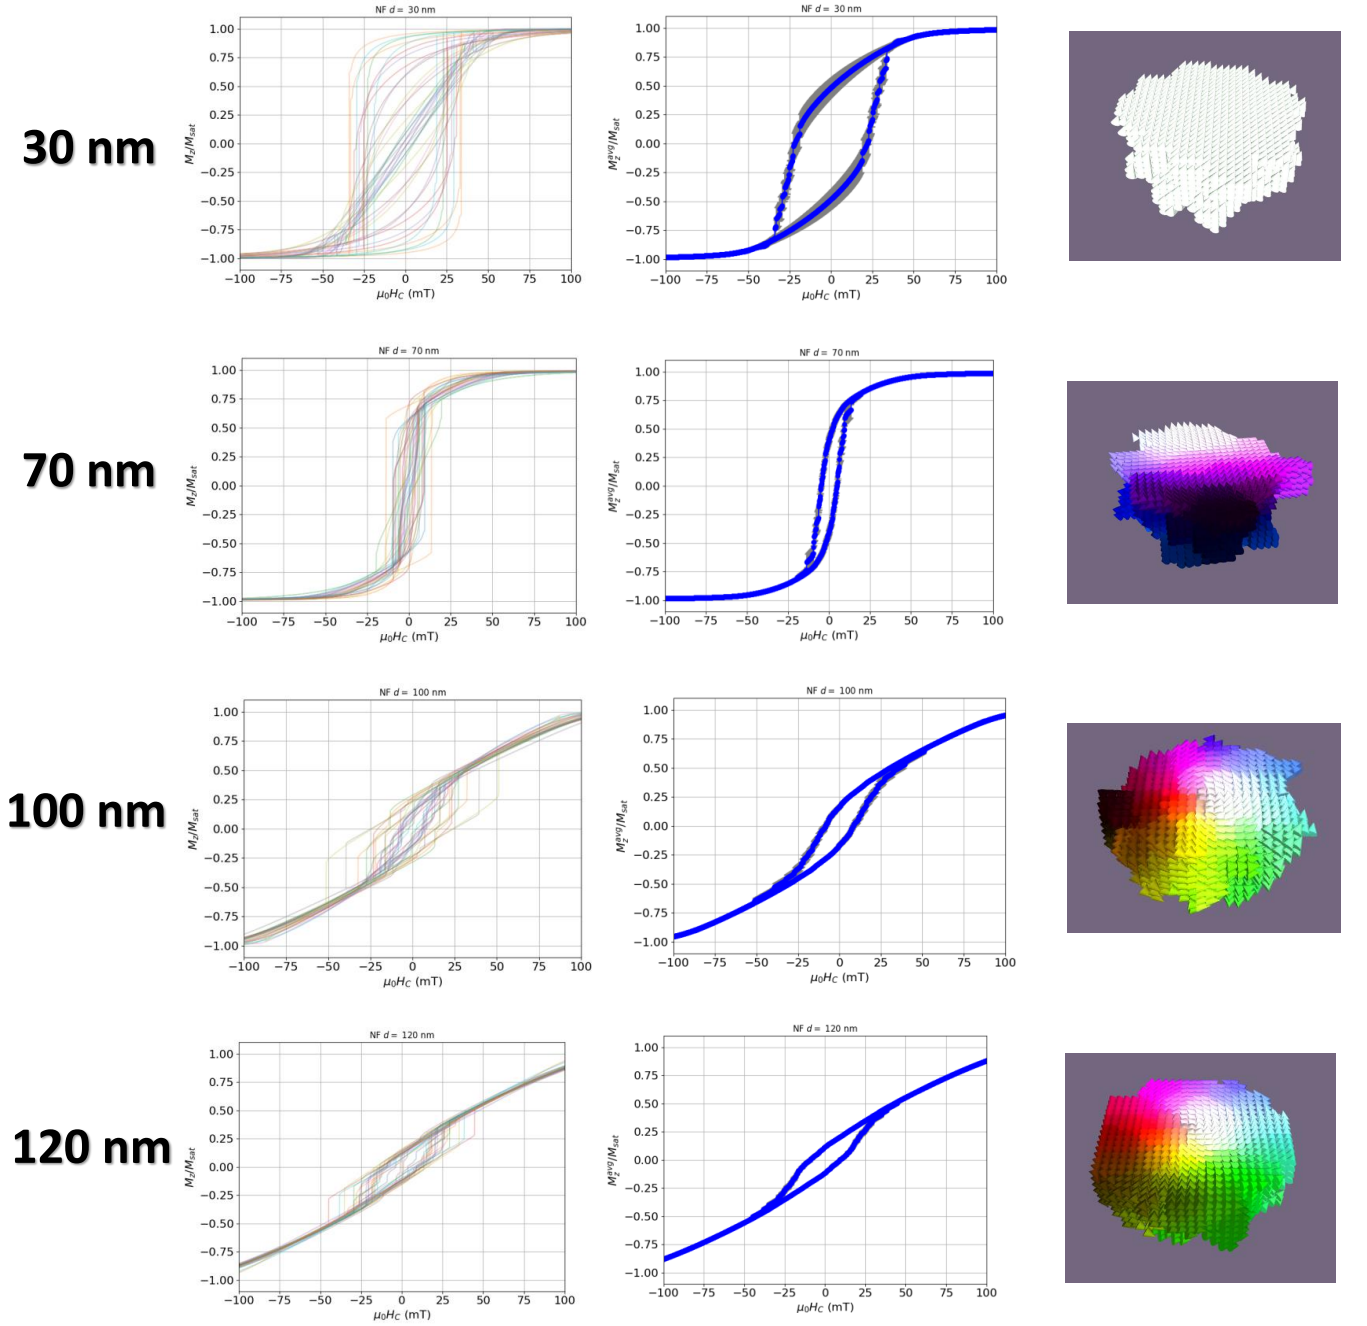

FIG. 1. Hysteresis loops for  $d = 30, 70, 100$ , and  $120$  nm NFs. Left column includes the loops of the 20 different realizations, each of them with a different random seed. The central column represents the averaged hysteresis loop from the individual realizations. The coercivity for each size in Fig. 1 of the main text is extracted from the averaged loops. Left column includes equatorial cuts of the remanent magnetization, illustrative of single domain ( $d = 30$  nm), domain wall ( $d = 70$  nm) and vortex ( $d = 100$  and  $120$  nm).

core or the in-plane flux-closure configuration dominates the magnetic structure. This dual mechanism becomes particularly evident in the idealized case of a perfect sphere (NS) with a single uniaxial anisotropy direction  $K_u$  along the field direction  $z$ , where the absence of intra-particle randomness allows to obtain exact results.

Moreover, Figure 2 of the main text detailed two reversal mechanisms, depending on whether the vortex core, or the flux-closure domains dominate the magnetization: one via a direct reversal of vortex core and the other by an intermediate rotation of the core in an

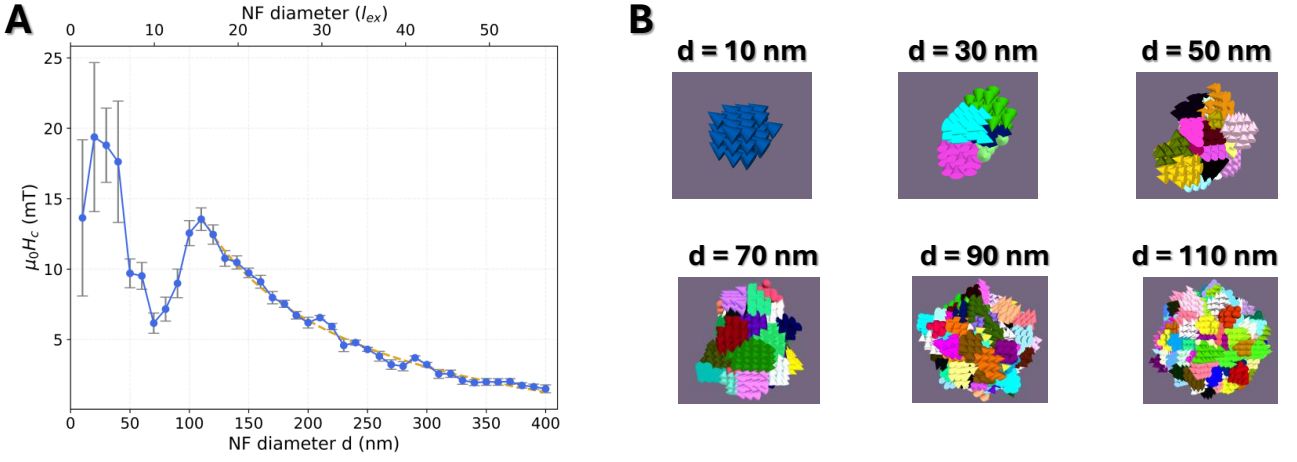

FIG. 2. **(A)** Coercivity as a function of NF diameter for all realizations with 15 nm grains. For diameters below 50 nm the error bars exceed 40 % because the nanoparticle is too small to accommodate 15 nm grains and maintain a quasi-spherical shape, occasionally yielding empty or incomplete geometries. **(B)** Representative NF geometries at the indicated diameters; colored arrows show the uniaxial anisotropy direction of each grain. The geometries up to  $d = 70$  nm appear unphysical, whereas the bottom row samples are sufficiently large to be unaffected by this artifact.

in-plane direction. The contrast between both reversal mechanisms is even more clear in an ideal sphere (NS) with a single easy axis  $K_u \parallel z$ , lacking any intra-particle disorder.

Figure 3**(A)** tracks the ratio  $V_{core}/V_{NS}$  as a function of the applied field (+ $z$  direction) for  $d = 100$  nm (dark-yellow circles),  $d = 110$  nm (purple squares), and  $d = 150$  nm (grey diamonds) representative of the core-dominated ( $d \leq 107$  nm) and in-plane (IP)-dominated ( $d \geq 108$  nm) regimes. At 100 mT, the ratio equals 1, meaning the nanoparticle is fully saturated. A drop from this value marks vortex nucleation. The larger magnetostatic field in larger spheres counteracts the uniform state favoured by the field. As a result, the vortex is stabilized at stronger external field for the larger NS (from  $\approx 40$  mT for  $d = 150$  nm, to 25 mT for  $d = 110$  nm, and 12 mT for  $d = 100$  nm). In every case the core volume shrinks as the field decreases.

For the core-dominated reversal ( $d = 100$  nm), the vortex never contracts below  $V_{core}/V_{NS} = 1/3$ . As a consequence, once the core flips, the in-plane moments gradually align with the field until full saturation is reached, and  $V_{core}/V_{NS}$  returns to 1. For  $d \geq 108$  nm, a two-step reversal mechanism appears. First, the core steadily contracts, until it reaches  $V_{core}/V_{NS} \approx 1/3$ . Then the magnetization rotates to bring a larger volume in alignment with the anisotropy easy axis, at the cost of the core lying perpendicular to both the field and easy axis. Close to the threshold diameter ( $d = 110$  nm) the anisotropy energy penalty is still large, and the vortex profile adapts by contracting the core further after it rotates, visible as the sharp drop in the purple curve. As  $d$  grows, the cost of a perpendicular core

decreases relative to the gain due to the alignment of the flux-closure moments with the anisotropy axis, producing a smoother  $V_{core}/V_{NS}$  profile (gray curve,  $d = 150$  nm).

The geometrical considerations of the  $V_{core}/V_{NS}$  determines the coercivity of the NS. Along with Figure 2 of the main text, we have analyzed the consequences of this ratio by studying the size-dependence of the polar angle  $\theta$  between the net NS magnetization and the + $z$  field, for the three sizes studied in Figure 3**(B)**.

For the core-dominated reversal ( $d = 100$  nm), the vortex core remains along  $z$  until its anisotropy barrier is crossed. Then, the entire magnetization flips sharply. In polycrystalline nanoflowers, however, multiple easy axes and grain boundaries can pin the core during reversal, thus some configurations briefly align the net moment perpendicular to the field, as observed in Figure 2 of the main text.

When the vortex core occupies less than one-third of the particle volume ( $V_{core} < 1/3$ ), the reversal is governed by the in-plane flux-closure moments. These moments encircle the core (initially along  $z$ ) and carry no net magnetization because rotational symmetry gives equal volumes magnetized along  $\pm x$  and  $\pm y$ . Once  $V_{core}$  drops below  $1/3$ , the combined magnetic volumes in the  $\pm x$  (or equivalently,  $\pm y$ ) direction exceed the core volume. Since uniaxial anisotropy depends only on the orientation of the magnetization and not on the sign of its direction, rotating the entire vortex profile by  $90^\circ$  (so the core tilts into the plane perpendicular to the field), becomes energetically favourable at low fields. The net moment therefore lies in the plane around

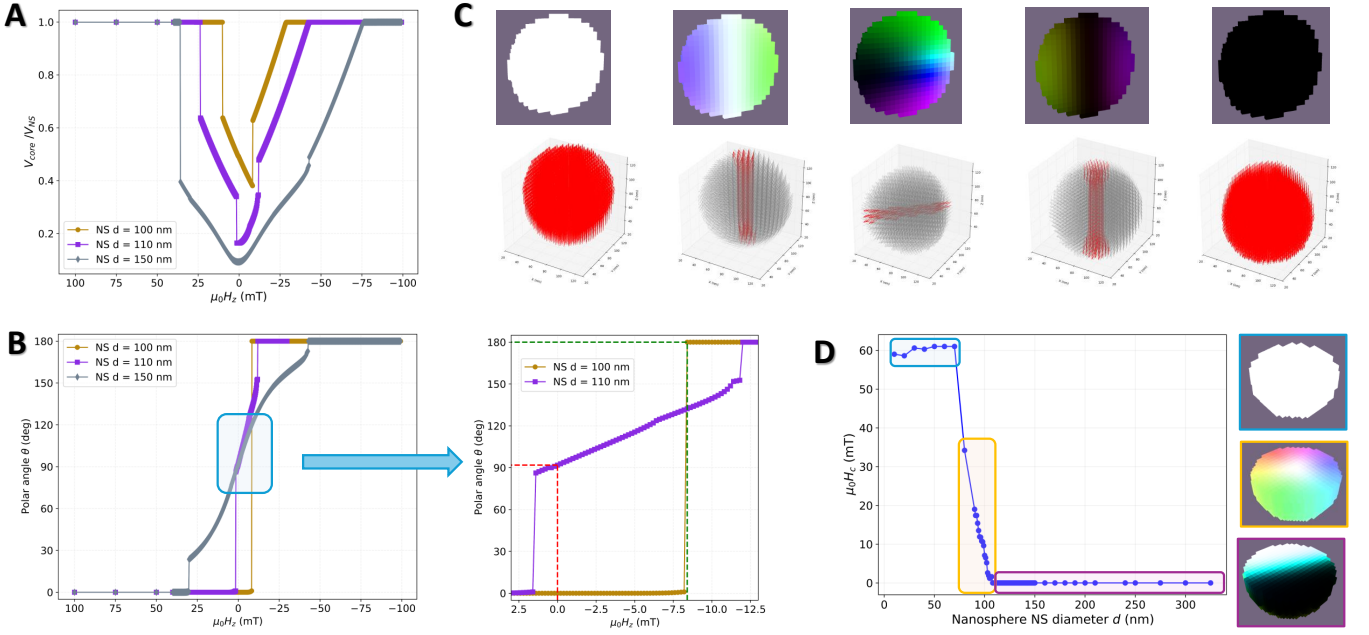

FIG. 3. **(A)** Field dependence of the volume ratio  $V_{core}/V_{NS}$  for nanospheres with  $d = 100$  nm (dark-yellow dots),  $d = 110$  nm (purple squares) and  $d = 150$  nm (gray diamonds); a pronounced drop near remanence appears for  $d \geq 108$  nm. **(B)** Polar angle  $\theta$  between the vortex core and the field axis as a function of the applied field  $\mu_0 H_z$  for the same cases as in **(A)**. The smaller sphere reverses by a sharp flip of the core along  $z$ . The right-hand side inset zooms-in the region close to remanence, marking by a green dashed line the switching of  $d = 100$  nm at  $\mu_0 H_z \cong -8.4$  mT; and a red dashed line marking the  $\theta \cong 90^\circ$  orientation of the net magnetization for  $d = 110$  nm at remanence which results in the zero coercivity of above  $d \geq 108$  nm. **(C)** Magnetization snapshots cuts along the  $y = 0$  plane for  $d = 110$  nm. Left and right extremes picture the saturation along  $+z$  (white) and  $-z$  (black), respectively. The left snapshot includes the initial vortex with the core along  $+z$ . Center: intermediate state with the core along  $x$ . Right: final state with the core along  $-z$ . **(D)** Coercivity versus NS diameter  $d$ , revealing three regimes: single domain (blue), vortex with core along  $z$  (dark-yellow), and vortex with core in-plane (purple). The right-hand side illustrates snapshots at remanence from the equatorial plane of the magnetization for  $d = 60$  nm,  $d = 100$  nm and  $d = 110$  nm, respectively.

remanence, as illustrated in Figure 3(A). The reversal becomes more gradual than in the core-dominated regime because the whole sphere now rotates as a single magnetic entity. This is even more evident for the larger NS ( $d = 150$  nm). To highlight the difference between both situations, we have zoomed-in the region around remanence in the right inset. Note how for  $d = 110$  nm, the polar angle is close to  $90^\circ$  at remanence (marked with a dashed red line), meaning the net magnetization is in-plane, and thus, yielding a 0 coercivity. The net magnetization for  $d = 100$  nm stays however along the  $z$  direction until  $\mu_0 H_z \cong -8.4$  mT, above its coercive field (see Figure 3(D)), and thus, the magnetization switches to the  $-z$  direction.

Figure 3(C) presents representative magnetization snapshots for  $d = 110$  nm to illustrate the full rotation process. The top row shows the  $y = 0$  slice, with the color representing the magnetization direction, while the bottom row emphasizes the vortex core in red. From left to right, the fields are  $\mu_0 H_z = -100, 2.0, 0, -11.8$  and  $100$  mT. The vortex core rotates smoothly out of the  $z$  axis, passing through

an intermediate state (middle frame at  $\mu_0 H_z = 0$  mT) that does not appear in the smaller particle.

Figure 3(D) plots coercivity versus the NS diameter. Three distinct regimes can be detected. For  $d < 93$  nm the nanosphere magnetization remains in a single-domain state, with uniform magnetization along  $+z$ , and  $\mu_0 H_C = 60$  mT. This result is slightly above the prediction of the Stoner Wollfarth model ( $\mu_0 H_C = 2K/M_s = 50$  mT). We verified that this mismatch can be ascribed to the grid anisotropy [14], which is expected for such highly symmetric perfect NS. For the irregular geometry of the NFs, this grid anisotropy just contributes as one more source of random anisotropy, i.e., it does not significantly alter our results. The single domain to vortex transition occurs at a larger diameter than the theoretical estimate  $d_{vortex} \approx \sqrt{2A/\mu_0 M_s^2} \approx 70$  nm  $\approx 10 \times l_{ex}$  [15–22]. The shift arises from the strong uniaxial anisotropy  $K_u$ , which disfavors the in-plane flux-closure pattern of the vortex and therefore requires a larger diameter before the demagnetizing energy can overcome the anisotropy energy.

For  $d \geq d_{vortex} = 93$  nm the NS adopts a vortex state: at remanence the core points along  $z$  and is encircled by in-plane flux-closure moments. As  $d$  grows, the core fraction  $V_{core}/V_{NS}$  shrinks and  $\mu_0 H_C$  falls accordingly. Once  $d > 107$  nm the flux-closure region outweighs the core, the vortex tilts into the plane perpendicular to  $z$ , and  $\mu_0 H_C$  drops to zero over the entire remaining size range.

## VI. INFLUENCE OF INTRA-PARTICLE DISORDER: CASE OF $k = 0$

In Section 3 of the main text we showed that coercivity depends on a balance between grain-boundary pinning

and the coherence of the vortex profile. To illustrate the limiting case, we simulated completely exchange decoupled grains ( $k = 0$ ). Figure 4 reveals the resulting magnetization: despite the remaining dipolar coupling between the grains, the coherence of the vortex profile is completely lost and instead a clear multi-domain pattern in which each grain behaves as an independent single-domain particle with its own random easy axis, is found. Averaging over these randomly oriented  $K_u$  directions drives the coercivity to zero. This extreme example highlights the essential role of inter-grain coupling in creating the hyperthermia “sweet spot”, where coercivity, and thus heating efficiency, is maximized.

- 
- [1] A. Vansteenkiste, J. Leliaert, M. Dvornik, M. Helsen, F. Garcia-Sanchez, B. Van Waeyenberge, *AIP Advances* **2014**, *4*, 10 107133.
  - [2] J. Leliaert, B. Van de Wiele, A. Vansteenkiste, L. Laurson, G. Durin, L. Dupré, B. Van Waeyenberge, *Journal of Applied Physics* **2014**, *115*, 23 233903.
  - [3] E. M. Jefremovas, L. Gandarias, I. Rodrigo, L. Marcano, C. Grüttner, J. Á. García, E. Garayo, I. Orue, A. García-Prieto, A. Muela, et al., *IEEE Access* **2021**, *9* 99552.
  - [4] C. Moya, M. Escoda-Torroella, J. Rodríguez-Álvarez, A. I. Figueroa, Í. García, I. B. Ferrer-Vidal, A. Gallo-Cordova, M. P. Morales, L. Aballe, A. F. Rodríguez, et al., *Nanoscale* **2024**, *16*, 4 1942.
  - [5] P. Bender, J. Fock, C. Frandsen, M. F. Hansen, C. Balceris, F. Ludwig, O. Posth, E. Wetterskog, L. K. Bogart, P. Southern, et al., *The Journal of Physical Chemistry C* **2018**, *122*, 5 3068.
  - [6] L. Storozhuk, M. O. Besenhard, S. Mourdikoudis, A. P. LaGrow, M. R. Lees, L. D. Tung, A. Gavrilidis, N. T. K. Thanh, *ACS Applied Materials & Interfaces* **2021**, *13*, 38 45870.
  - [7] H. Gavilán, E. H. Sánchez, M. E. Brollo, L. Asín, K. K. Moerner, C. Frandsen, F. J. Lázaro, C. J. Serna, S. Veintemillas-Verdaguer, M. P. Morales, et al., *ACS omega* **2017**, *2*, 10 7172.
  - [8] A. G. Roca, J. F. Marco, M. d. P. Morales, C. J. Serna, *The Journal of Physical Chemistry C* **2007**, *111*, 50 18577.
  - [9] H. Shokrollahi, *Journal of Magnetism and Magnetic Materials* **2017**, *426* 74.
  - [10] E. P. Sinaga, M. P. Adams, E. H. Hasdeo, A. Michels, *Physical Review B* **2024**, *110*, 5 054404.
  - [11] B. Gross, S. Philipp, E. Josten, J. Leliaert, E. Wetterskog, L. Bergström, M. Poggio, *Physical Review B* **2021**, *103*, 1 014402.
  - [12] J. Borchers, K. Krycka, B. Bosch-Santos, E. de Lima Correa, A. Sharma, H. Carlton, Y. Dang, M. Donahue, C. Grüttner, R. Ivkov, et al., *Small Structures* **2025**, *6*, 2 2400410.
  - [13] K. Pisane, S. Singh, M. Seehra, *Applied Physics Letters* **2017**, *110*, 22.
  - [14] S. J. Holt, A. Petrocchi, M. Lang, S. A. Pathak, H. Fangohr, *arXiv preprint arXiv:2412.10466* **2024**.
  - [15] M. E. Schabes, H. N. Bertram, *Journal of Applied Physics* **1988**, *64*, 3 1347.
  - [16] R. Hertel, H. Kronmüller, *Journal of magnetism and magnetic materials* **2002**, *238*, 2-3 185.
  - [17] W. Rave, K. Fabian, A. Hubert, *Journal of Magnetism and Magnetic Materials* **1998**, *190*, 3 332.
  - [18] A. R. Muxworthy, W. Williams, A. P. Roberts, M. Winklhofer, L. Chang, M. Posfai, *Geochemistry, Geophysics, Geosystems* **2013**, *14*, 12 2430.
  - [19] D. Betto, J. Coey, *Journal of Applied Physics* **2014**, *115*, 17.
  - [20] W. Gan, M. Chandra Sekhar, D. Wong, I. Purnama, S. Chiam, L. Wong, W. Lew, *Applied Physics Letters* **2014**, *105*, 15.
  - [21] A. Kákay, L. Varga, *Journal of applied physics* **2005**, *97*, 8.
  - [22] A. Witt, K. Fabian, U. Bleil, *Earth and Planetary Science Letters* **2005**, *233*, 3-4 311.

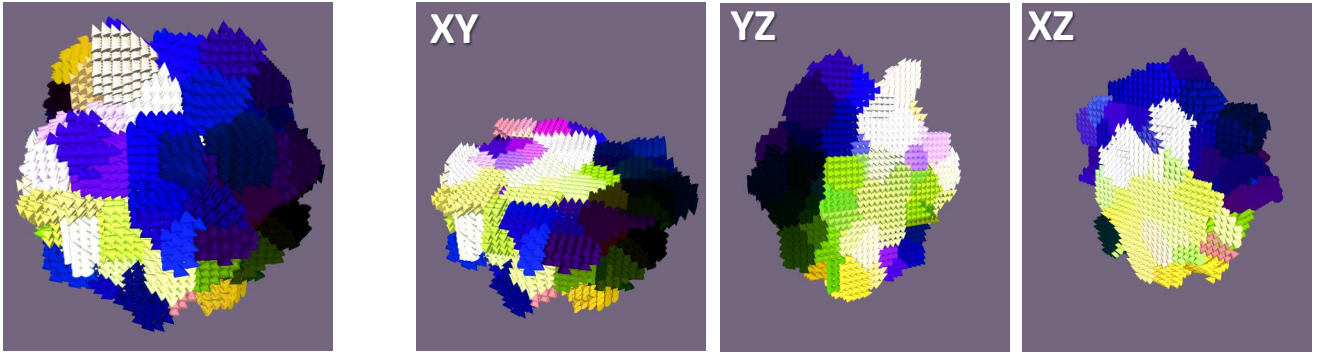

FIG. 4. Remanent magnetization distributions, shown for a  $d = 100$  nm NF with exchange uncoupled grains ( $k = 0$ ), along with the corresponding three central planes  $XY$ ,  $YZ$  and  $XZ$ . Each color represents a different magnetization direction, illustrating the uncoupled, multi-domain magnetization state.
